# Supplementary material for: Connecting quantum circuit amplitudes and matrix permanents through polynomials
Source: arXiv:2408.08857 source file (2024-08-16)
Supplement: Supplementary file 1 [file framework.tex]

\section{Framework} \label{app:framework}

In his work, Rudolph \cite{rudolph_simple_2009} proposes a method to encode the
amplitudes of quantum circuits built upon the gates Hadamard and Toffoli as
permanents of the adjacency matrices associated to graphs -- or more loosely,
permanents of graphs. To achieve this, the circuit is first associated to a low
degree polynomial $f$ over $\mathbb F_2$ and each clause of that polynomial is
associated with a graph gadget. The individual gadgets are then linked together
with cycles representing the variables they share to form the final graph.
Reading the permanent of a graph as the sum of the weights of its cycle covers
allows one to interpret the permanent as a sum over the assignments of the
variables. Computing the graph permanent of $G$ therefore \emph{bruteforces} the
computation of the exponential sum
\begin{equation}
    \per G = \sum_{\substack{\x \in \{0, 1\}^{n}}}(-1)^{f(\x)},
\end{equation}
by computing the value of each cycle cover. The weight of a \emph{valid} cycle
cover corresponds to one of the $(-1)^{f(\x)}$ using the following rule
mentioned in the main text: in a particular cycle cover, the absence of a cycle
corresponding to a variable corresponds to the fact that the variable is
assigned the value 1, and its presence corresponds to its assignment to 0.
However, notice that not all cycle covers correspond to a valid assignment of
the variables, see example in \autoref{fig:validInvalidCoverApp}. The bold blue
edges represent the cycles associated to variables.
% \begin{figure}[hbtp!]
%     \centering%
%     \begin{subfigure}[t]{.45\textwidth}%
%         \centering%
%         \input{img/valid_cycle_cover.tex}
%         \caption{\emph{Valid} cycle cover. Say vertex 1 is connected to the
%         variable $x$ and 2 to $y$, then the cycle cover assigns $x = 0$ and $y =
%         1$, and the contribution of the gadget is $(-1)^{xy} = 1$.}
%         \label{fig:validCoverApp}
%     \end{subfigure}\hfill%
%     \begin{subfigure}[t]{.45\textwidth}
%         \centering
%         \input{img/invalid_cycle_cover.tex}
%         \caption{\emph{Invalid} cycle cover. The overall contribution of such
%         covers must be zero. See example of
%         \autoref{fig:quadraticGadgetsCrossingPaths}.}
%         \label{fig:invalidCoverApp}
%     \end{subfigure}
%     \caption{Illustrative example of the gadget representing the quadratic clauses
%     of the polynomial from \cite{rudolph_simple_2009}. Example of a cycle cover
%     corresponding to a valid assignment of the variable in \autoref{fig:validCoverApp}
%     and an invalid one in \autoref{fig:invalidCoverApp}.}
%     \label{fig:validInvalidCoverApp}
% \end{figure}

The covers that traverse a cycle corresponding to a variable cannot be
associated with a consistent assignment of that variable, therefore their
contributions should interfere destructively and sum up to zero. An example of
such cancellation is given in \autoref{fig:quadraticGadgetsCrossingPaths}. The
properties of the polynomial are direct consequence of its encoding. It is a
polynomial of degree 3, in which each variable that appears in a cubic clause
must then appear in two quadratic clauses. This property is ensured by
construction: each target of the Toffoli gates must be followed by a pair of
Hadamard gates hence the degree is bounded. This additional, necessary structure
ensures that quadratic clause gadgets suffice to \emph{force} an external edge
which is incident to the cubic clause gadget to leave via the same vertex it
entered. Therefore, a simpler cubic clause gadget can be used, as it does not
have to satisfy these constraints on the cycle covers, and no gadget for clauses
of degree higher than 3 is needed. The major drawback is that the pair of
Hadamard gates, used to bound the degree, is required even when the degree does
not have to be bounded. This is the case for IQP circuits, which are the focus
of this work \cite{montanaro_quantum_2017}.

\begin{figure}[hbtp!]
    \centering
    \begin{subfigure}{.45\textwidth}
        \centering
        \input{img/quadratic_gadget_crossing_paths_1.tex}
        \caption{Part of a crossing cycle.}
        \label{fig:crossPath1}
    \end{subfigure}\hfill%
    \begin{subfigure}{.45\textwidth}
        \centering
        \input{img/quadratic_gadget_crossing_paths_2.tex}
        \caption{Part of another crossing cycle.}
        \label{fig:crossPath2}
    \end{subfigure}
    \caption{Illustrative example of the gadget representing the quadratic clauses
    of the polynomial from \cite{rudolph_simple_2009}. The blue edges correspond to
    cycles representing the variables. The gadget design must be so that each
    crossing path can be paired with another with contribution of opposite sign to
    the cycle cover in a way which causes the necessary cancellation. In this
    instance, the contribution depicted in \autoref{fig:crossPath1} is cancelled by
    the one shown in \autoref{fig:crossPath2}.}
    \label{fig:quadraticGadgetsCrossingPaths}
\end{figure}
